# Supplementary material for: Statistical modeling of the gas-liquid interface using geometrical variables: toward a unified description of the disperse and separated phase flows
Source: arXiv:1710.04585 source file (2017-10-13)
Supplement: Supplementary file 1 [file appendice1.tex]

Using the equations \eqref{eq:ASDF-requirement1}, \eqref{eq:ASDF-requirement2_3}, \eqref{eq:aaverg} and \eqref{eq:paverg} in the spatial-averaged SDF \eqref{eq:ASDF}, we fulfil the three properties discussed above. However, these equations are not simple to interpret and can introduce more complexities and difficulties in modeling the unclosed terms of the GPBE satisfied by the SDF. Therefore, we propose two simplified averaged SDFs, which do not satisfy all the requirements but which can be more simple to use in the modeling and physical interpretation. For the first one, we use the same equation \eqref{eq:ASDF}, \eqref{eq:aaverg} and \eqref{eq:paverg} but the kernel function is defined as follows:
\begin{equation}
w(\xv;\rv)=\begin{cases}
  0 & \text{if  $||\rv||>h$} \\
  \dfrac{1}{\vol_h}, & \text{otherwise}
  \end{cases}
\end{equation}
where $\vol_h$ is the volume of the set point $\{\rv'\in\mathrm{R}^3,\,\, ||\rv'||<h\}$. The averaged SDF in this case can be written simply as follows:
\begin{equation}
\ASDF(t,\xv;\phasevar)=<\dfrac{S_h(t,\xv)}{\vol_h}\delta(\phasevar-\aaverg{\phasevar}(t,\xv))>
\label{eq:ASDF2}
\end{equation}
where $S_h(t,\xv)=\int_{\yv\in\Volh{\xv}}\delta_I(\yv)\dint{3}{\yv}$ is the area of the surface included in the volume space $\Volh{\xv}$, and the averaged interfacial variables are given by:
\begin{equation}
\paverg{\phasevar}(t,\xv)=\dfrac{1}{S_h(t,\xv)}\int_{\yv\in\Volh{\xv}}\delta_I(\yv)\phasevar(\yv)\dint{3}{\yv}
\end{equation}
The SDF given in \eqref{eq:ASDF2} does not satisfy the first requirement \ref{item:requirement1}, and the second requirement \ref{item:requirement2} can be interpreted in another way, which we will discuss later. The second average SDF, which we propose, reads:
\begin{equation}
\ASDF(t,\xv;\phasevar)=<\delta_I(\xv)\delta(\phasevar-\paverg{\phasevar}(t,\xv))>
\label{eq:ASDF3}
\end{equation}
this time only the interfacial quantities have been spatially-averaged and we keep the same area measure as for the general SDF. This basic averaged SDF satisfies the first and the third requirements but it does not satisfy the conservation of topological information in general case (disperse and separated phases), described in \ref{item:requirement2}. In the following, we adopt the first definition, since it provides a consistent definition of the averaged SDF and satisfies the three required properties. However, for future work and especially if we would to interest to close the equations, it can be more convenient to use one the two last simplified averaged SDF. In the results section, we will compare the two last SDF and we will give an other interpretation of the third requirement in the case of the averaged SDF given in \eqref{eq:ASDF2}.
